# Supplementary material for: Coin Flipping of \emph{Any} Constant Bias Implies One-Way Functions
Source: arXiv:2105.01400 source file (2021-05-04)
Supplement: Supplementary file 1 [file AdditionalProperties.tex]

\remove{
In the previous section we  proved that  the iterated biased-continuation attacker  breaks any coin-flipping protocol with bias arbitrarily close to $\frac12$. The goal of this section is to implement the biased-continuation attacker \emph{efficiently}, assuming one-way functions do not exist.

Let us start with an informal discussion. Given a protocol $\cpi = (\Ac,\Bc)$, define its  ``transcript" function $f= f_\cpi$ by
$$f(r_\HonA,r_\HonB,i)=\trans(\HonA(r_\HonA),\HonB(r_\HonB))_{1,\ldots,i}.$$
Namely, given the randomness of the parties and a round index, $f$ outputs the transcript up to this round. Assuming one-way functions do not exist, then $f$ has a $\gamma$-inverter $\Inv_f$ for any $\gamma(n) \geq 1/\poly(n)$ (\ie the output of $\Inv_f$  is $\gamma$ close to an ideal inverter for $f$). We can now try and implement the  biased-continuation attacker for $\cpi$  using such $\gamma$-inverter $\Inv_f$: to implement the attack of  $\rcA{1}$ on a node $u$, call $\Inv_f$ many times until it outputs $(r_\HonA,r_\HonB,|u|)$ such that $\out(\HonA(r_\HonA),\HonB(r_\HonB))=1$, and use this randomness to compute the next message of $\Ac$.

Unfortunately, when trying to implement the above approach, one faces two problems. The first (which also holds for the case of an ideal inverter) is that there might be nodes whose value is so low that the number of times the inverter has to be called is too large. The second is that a $\gamma$-inverter for $f$ is only guaranteed to work well  on \emph{average} --- on the output distribution  of $f$ (\ie a random transcript of $(\HonA,\HonB)$). The queries made by the biased-continuation attacker, however,  might be distributed very far from the latter distribution. In particular, it might be the case that there are some nodes that are visited in $(\rcA{1},\HonB)$ with much higher  probability than in $(\HonA,\HonB)$. We call such nodes ``unbalanced", and note that a $\gamma$-inverter for $f$ gives no guarantee on them.

The key observation in this section is that  a random execution of $(\rcA{1},\HonB)$ almost never visits an unbalanced node without first visiting a low value node (\cref{sec:BiassCOntAdditionalProp}). The same can be generalized to any constant number of recursions. Hence, if we are given a protocol that is guaranteed not to have low-value nodes controlled by $\HonA$ and high-value nodes controlled by $\HonB$, then the above natural approach works well enough. %Namely, we can (almost) directly apply the theorem of the previous section.

\remove{It might sound paradoxical, but in such protocols recursive biased-continuation attack does very well in biasing the outcome of the protocol, but at the same time it does so by not changing the transcript distribution by a lot. \footnote{This is not a discrepancy. Take for example any protocol and condition on not hitting a 0-leaf. The resulting conditional protocol has value 1 (roughly speaking this is like a perfect attack) and no node has more than twice as much weight as in the original protocol. Therefore no node is really unbalanced.}}

The next step is to efficiently convert an arbitrary protocol, to one with no $\HonA$'s control low value nodes and with no $\HonB$'s control high-value nodes. This can be achieved (\cref{sec:PrunedProtcol}) by having the two parties check the value of each node they visit. Once they find out that a node has low [resp. high] value (\eg smaller than some) $\delta$ [resp. larger than $1-\delta$], then $\HonB$ [resp. $\HonA$] takes control and decides the output of the protocol in a way that does not change the value of the node. We denote the resulting ``pruned" protocol by $\cpi_\delta=(\HonA_\delta,\HonB_\delta)$. Note that in this pruned protocol,  the biased-continuation attacker $\HonA_\delta^{(1)}$ does not call the inverter on low-value nodes.

While  implementing the above pruned  protocol might be infeasible, using the transcript  function inverter for $\cpi$, one can implement an ``approximately pruned'' variant of $\cpi$. Specifically, we show that if the probability of hitting a node whose value is close to the threshold $\delta$ in $\cpi$ is low, then the transcripts of $\cpi_\delta$ and $\widetilde{\cpi}_\delta$ are statistically close, where $\widetilde{\cpi}_\delta$ is the approximately pruned variant of $\cpi$ (\cref{sec:PrunedProtcol}). The latter is in use, since we show the following  robustness property of the biased-continuation attack (\cref{subsec:Robustness}): in case the transcript distributions of two protocols are statistically close, then it is also the case for the protocols resulting from  applying biased-continuation attack on each of these protocols. We show that there exists $\delta'$, chosen from a polynomial size thresholds list, all close to $\delta$, such that the probability of hitting a node whose value is close to $\delta'$ is small. It follows that the biased-continuation attack does almost as well on the pruned  protocol and on its approximated variant.
%. \footnote{For ease of presentation, the implementation of the approximated pruned variant of the protocol is stateless, because this way the biased-continuation attack can be implemented very easily. }

 Before iterating the approximated biassed-continuation attack on the above  approximately pruned protocols, there is still one issue to be taken care of. As the inverter is not perfect, after the first iteration there might be nodes whose values are high in the original protocol, but low after a single recursion. As we do not know what is the probability of hitting such a node, we can not safely apply second recursion. We handle this problem by having the attacker, which we call the "pruning attacker", prune the protocol at low value nodes before each further recursion and show that the resulting transcript distribution is still close to $(\HonA^{(k)}_\delta,\HonB_\delta)$ (\cref{sec:PruningAttack}).

We explained above that the iterated approximated biassed-continuation attacker,  successfully attacks the approximately pruned protocols. But why should it help us for attacking the actual (non pruned) protocol? The key point is that we can have our final attacker use this ``pruned" attacker in \emph{its head}, while interacting with $\HonB$ (\cref{sec:finalAppx}). We call this attacker the ``pruning-in-the-head attacker". The pruned attacker dictates  how the pruning-in-the-head attacker should act up to the point they reach a low or high value node. Once the pruning-in-the-Head attacker and $\HonB$ reach such a node, the former starts behaving honestly. This does not deteriorate the success probability of the pruned attacker too drastically because (a) after seeing a low-value node the pruned attacker expects the other party to decide on the outcome and honest behavior actually emulates exactly that; and (b) once high-value node is hit, honest execution of its own implies high probability of outputting $1$.

We start, in \cref{sec:BiassCOntAdditionalProp}, by observing additional properties of the (ideal) biased-continuation attacker (defined in \cref{sec:IdealAttacker}), in particular the property regarding the probability of visiting unbalanced nodes and the robustness property. In \cref{subset:BasicTools}, we define the basic tools to be used by our efficient attackers, and show that in some scenarios these tasks can be implemented efficiently. In \cref{sec:EfficientRCAttacker}, we consider an approximated variant of the ideal biased-continuation attacker. In \cref{sec:PrunedProtcol}, we define the pruned variant of a protocol (both ideal and approximated), where in \cref{sec:PruningAttack} we present the "pruning attacker". In \cref{sec:finalAppx}, we present the "pruning-in-the-head attacker" for \emph{any} protocol, where finally, in \cref{subsec:EfficeinrAttack} we present the efficient implementation of the latter pruning attacker, under the assumption that one-way functions do not exist.

Throughout this section, we assume for simplicity that the last message sent in a protocol is its output bit (recall that we restricted our attention to protocols in which both parties always output the same bit value). As in \cref{sec:IdealAttacker}, the attackers described below taking the left hand side party of the protocol (i.e., $\HonA$), are trying to bias the common output of the protocol towards one where the attackers
taking the right hand side party (i.e., $\HonB$) are trying to bias the common output towards zero.
}%end remove

\section{Additional Properties of the Biased-Continuation Attack}\label{sec:BiassCOntAdditionalProp}

\subsection{Robustness}\label{subsec:Robustness}
The following lemma states that, under a certain condition,
